# Supplementary material for: Dissipative Floquet Majorana modes in proximity-induced topological superconductors
Source: arXiv:2004.14918 source file (2021-03-06)
Supplement: Supplementary file 1 [file SM_v3.pdf]

# Supplementary Material for “Dissipative Floquet Majorana modes in proximity-induced topological superconductors”

## CONTENTS

|                                                                    |   |
|--------------------------------------------------------------------|---|
| I. Derivation of the Floquet Retarded Green's Function             | 1 |
| II. Recursive Green's Function Method                              | 2 |
| III. Some additional notes of the Majorana poisoning model         | 3 |
| A. The definition of lifetime                                      | 4 |
| 1. Review the definition of lifetime based on the Green's function | 4 |
| 2. Some insights of the Majorana poisoning model                   | 5 |
| 3. Definition of lifetime                                          | 6 |
| B. The lifetime of the Floquet Majoranas in different Floquet BZs  | 7 |
| C. The differences between the peaks in different Floquet BZs      | 7 |
| References                                                         | 7 |

## I. DERIVATION OF THE FLOQUET RETARDED GREEN'S FUNCTION

In this section, we will briefly show how to derive  $G_{nw}^R(k, \omega)$ .

The Green's function in our driven-dissipative system can be defined as

$$G_{nw}^R(k; t, t') = -i\theta(t - t')\langle\{\psi(k, t), \psi^\dagger(k, t')\}\rangle, \quad (1)$$

where  $\psi(k, t) = (c_\uparrow(k, t), c_\downarrow(k, t), c_\uparrow^\dagger(-k, t), c_\downarrow^\dagger(-k, t))^t$ . The Fourier transformation for  $\psi(k, t)$  in a periodical driving system can be expressed as

$$\psi(k, t) = \sum_m \int_{-\Omega/2}^{\Omega/2} \frac{d\omega}{2\pi} e^{-i(\omega+m\Omega)t} \psi_m(k, \omega). \quad (2)$$

Then the Fourier transformation for the Green's function  $G_{nw}^R(k; t, t')$  will be[1]:

$$G_{nw}^R(k; t, t') = \sum_{mn} \int_{-\Omega/2}^{\Omega/2} \frac{d\omega}{2\pi} e^{-i(\omega+m\Omega)t+i(\omega+n\Omega)t'} \left[ \underline{G_{nw}^R(k, \omega)} \right]_{mn}, \quad (3)$$

and

$$\left[ \underline{G_{nw}^R(k, \omega)} \right]_{mn} = \frac{1}{T} \int_0^T dt_{av} \int_{-\infty}^{\infty} dt_{rel} e^{i(\omega+m\Omega)t - i(\omega+n\Omega)t'} G_{nw}^R(k; t, t'), \quad (4)$$

where  $t_{av} = \frac{1}{2}(t + t')$  and  $t_{rel} = t - t'$ .

After integrating out the SC bath degrees of freedom, the influence provided by the SC bath can be expressed by the self-energy  $\Sigma_{sc}(t)$ . Since the SC bath doesn't be driven, the Fourier transformation of the self-energy provided by it is still the original one

$$\Sigma_{sc}(\omega) = \int dt e^{-i\omega t} \Sigma_{sc}(t), \quad (5)$$

where  $\Sigma_{sc}(\omega) = V^2 \sigma_z \tau_0 [\hat{q}_{bath}^R(\omega)] \sigma_z \tau_0$  and  $\hat{q}_{bath}^R(\omega)$  is the retarded quasi-classical Green's function[2, 3] of the SC bath. Here we briefly show the derivation of  $\hat{q}_{bath}^R(\omega)$ .

The Nambu-Gor'kov Green's function in the Matsubara formalism can be expressed as

$$\mathcal{G}(k, i\omega_n) = \frac{1}{(i\omega_n)^2 - (\epsilon_k^2 + \Delta^2)} \begin{pmatrix} i\omega_n + \epsilon_k & \Delta \\ \Delta & i\omega_n - \epsilon_k \end{pmatrix}. \quad (6)$$

Analytical continuation  $\omega_n \rightarrow -i(\omega + i\eta)$  leads to the retarded Green's function in the real frequency space

$$\mathcal{G}^R(k, \omega) = \frac{1}{(\omega + i\eta)^2 - (\epsilon_k^2 + \Delta^2)} \begin{pmatrix} \omega + i\eta + \epsilon_k & \Delta \\ \Delta & \omega + i\eta - \epsilon_k \end{pmatrix}. \quad (7)$$

As the quasi-classical Green's function is defined as  $\hat{q}_{bath}^R(\omega) = \rho_F \int d\epsilon_k \mathcal{G}_{bath}^R(k, \omega)$ , where  $\rho_F$  is the DoS in the vicinity of the Fermi surface, then residual theorem leads to

$$\hat{q}_{bath}^R(\omega) = -i\pi\rho_F \frac{1}{\sqrt{(\omega + i\eta)^2 - \Delta^2}} \begin{pmatrix} \omega + i\eta & \Delta \\ \Delta & \omega + i\eta \end{pmatrix}. \quad (8)$$

Matrices in our consideration are in BdG space, so we have

$$\begin{aligned} \hat{q}_{bath}^R(\omega) &= \pi\rho_F \frac{1}{\sqrt{-(\omega + i\eta)^2 + \Delta^2}} \begin{pmatrix} -(\omega + i\eta) & 0 & 0 & -\Delta \\ 0 & -(\omega + i\eta) & \Delta & 0 \\ 0 & \Delta & -(\omega + i\eta) & 0 \\ -\Delta & 0 & 0 & -(\omega + i\eta) \end{pmatrix} \\ &= \pi\rho_F \frac{1}{\sqrt{-(\omega + i\eta)^2 + \Delta^2}} [-(\omega + i\eta) + \Delta\sigma_y\tau_y]. \end{aligned} \quad (9)$$

Since the value of  $\rho_F$  doesn't matter in our problem, we can simply let  $\pi\rho_F = 1$ . Therefore,

$$\Sigma_{sc} = V^2 \frac{1}{\sqrt{-(\omega + i\eta)^2 + \Delta^2}} [-(\omega + i\eta) - \Delta\sigma_y\tau_y]. \quad (10)$$

Together with the non-dissipative Floquet Hamiltonian, one can define the Floquet Green's function in the frequency space as

$$\underline{G}_{nw}^R(k, \omega) = \frac{1}{\underline{\omega} - \underline{H}_{nw}(k) - \underline{\Sigma}_{sc}(\omega)}, \quad (11)$$

where the non-dissipative Floquet Hamiltonian reads as

$$\underline{H}_{nw}(k) = \begin{pmatrix} \dots & & & & \\ & \mathcal{H}_{nw}(k) - \Omega & A\sigma_0\tau_z & 0 & \\ & A\sigma_0\tau_z & \mathcal{H}_{nw}(k) & A\sigma_0\tau_z & \\ & 0 & A\sigma_0\tau_z & \mathcal{H}_{nw}(k) + \Omega & \\ & & & & \dots \end{pmatrix}, \quad (12)$$

,  $[H_{nw}(k)]_{mm'} = \frac{1}{T} \int_0^T dt e^{i(m-m')\Omega t} H_{nw}(k, t)$  and  $H_{nw}(k, t) = ((-2t \cos k - \mu_0 + 2A \cos \Omega t)\sigma_0 + V_z \sigma_z + \lambda \sin k \sigma_y)\tau_z$ . Let  $\underline{\mathcal{H}}_{eff}(k, \omega) = \underline{H}_{nw}(k) + \underline{\Sigma}_{sc}(\omega)$ , we then get the expression of  $\underline{G}_{nw}^R(k, \omega)$ :

$$\underline{G}_{nw}^R(k, \omega) = [\underline{\omega} - \underline{\mathcal{H}}_{eff}(k, \omega)]^{-1}. \quad (13)$$

Our numerical calculation is based on Eq.(13). We truncate  $\underline{\mathcal{H}}_{eff}(k, \omega)$  and just leave a  $(21 \times 4) \times (21 \times 4)$  matrix ( $N_F = 21$ ), then numerically calculate  $\underline{G}_{nw}^R(k, \omega)$ . Finally, calculating  $\nu_k(\omega)$  through Eq. (6) in the main body of this letter leads us to Fig. 2(a) in the main body.

## II. RECURSIVE GREEN'S FUNCTION METHOD

This section will show how to get Fig. 2(b) in the main body through the recursive Green's function method. For details of the recursive Green's function method, we refer to Ref. [4–6]. In our problem, Green's functions are more structured due to the introducing of Floquet and Keldysh space.

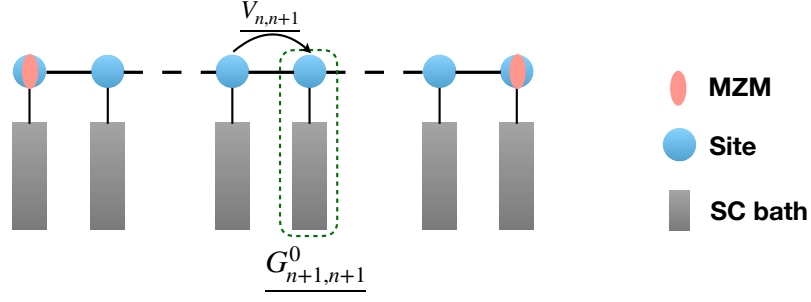

FIG. 1. Lattice model for recursive Green function method. We suppose the nanowire is composed by 200 sites, and couple an identical SC bath to each site.

The key to using the recursive Green's function method is to regard the nanowire as a lattice model (see Fig. 1). We suppose that this nanowire has 200 sites. Since we just care about the energy spectrum and use the SC bath to produce an induced gap for the nanowire, the correlation in the bath can be ignored under Markovian approximation. In this case, and the influence on each site from the SC bath are the same, which equals to that we couple an identical SC bath to each site.

In order to detect MZMs localized in two edges of this wire, we use the following recursive equation:

$$\underline{G}_{n+1,n+1}^d(\omega) = [\underline{G}_{n+1,n+1}^0(\omega) - \underline{V}_{n+1,n} \cdot \underline{G}_{n,n}^d(\omega) \cdot \underline{V}_{n,n+1}]^{-1} \quad (14)$$

where  $\underline{V}_{n,n+1}$  denotes the hopping term between  $n$ th and  $(n+1)$ th site in the Floquet $\otimes$ Keldysh $\otimes$ BdG space, the subscript  $n$  denotes the  $n$ th site, and the superscript  $d$  and  $0$  denote the dressed Green's function of one site after considering the hopping term  $\underline{V}_{n,n+1}$  and the bare Green's function of one site with only the onsite energy, respectively. Note that  $\underline{G}_{1,1}^d(\omega) = \underline{G}_{1,1}^0(\omega)$ . After 199 recursions, one will get  $\underline{G}_{200,200}^d(\omega)$ . Then using Eq. (9) in the main body of this letter will lead us to Fig. 2(b) in the main body of this letter.

### III. SOME ADDITIONAL NOTES OF THE MAJORANA POISONING MODEL

In this section, we provide some additional calculations and notes of the Majorana poisoning model. Starting from the effective Hamiltonian,

$$\underline{H}(\omega) = \begin{pmatrix} \cdots & \Sigma(\omega + \Omega) - \Omega & A & 0 \\ & A & \Sigma(\omega) & A \\ & 0 & A & \Sigma(\omega - \Omega) + \Omega \\ & & & \cdots \end{pmatrix}, \quad (15)$$

where

$$\Sigma(\omega) = -V^2(\omega + i\eta)/\sqrt{-(\omega + i\eta)^2 + \Delta^2}. \quad (16)$$

Here  $A$ ,  $V$ ,  $\Delta$  represent the driving amplitude, Majorana-bath coupling strength, and driving frequency, respectively. The major feature of this effective model is that the Hamiltonian is energy dependent, due to the existence of self-energy correction,  $\Sigma(\omega)$ . Since for a given  $\omega$ ,  $H(\omega)$  is non-Hermitian, it is convenient to introduce the biorthogonal basis,

$$\underline{H}(\omega)|u_m^R(\omega)\rangle = E_m(\omega)|u_m^R(\omega)\rangle, \quad \langle u_n^L(\omega)|\underline{H}^\dagger(\omega) = E_n(\omega)\langle u_n^L(\omega)|$$

where  $\langle u_n^L(\omega)|u_m^R(\omega)\rangle = \delta_{nm}$ . Based on this basis, one can express the matrix element of the retarded Green's function in the Floquet space,

$$[\underline{G}^R(\omega)]_{mn} = \langle m|\frac{1}{\underline{\omega} - \underline{H}(\omega)}|n\rangle = \sum_s \frac{\langle m|u_s^R(\omega)\rangle\langle u_s^L(\omega)|n\rangle}{\omega - E_s(\omega)}, \quad (17)$$

where  $m, n, s$  represent the Floquet sites. The time-averaged DoS is defined as the 00-entry of the retarded Green's function defined in the Floquet space, namely,

$$\nu(\omega) = -\frac{1}{\pi} \text{Im} \left[ \overline{G^R(\omega)} \right]_{00}, \quad (18)$$

The corresponding propagator is defined as

$$G^R(t, t') = \sum_{mn} \int_{-\Omega/2}^{\Omega/2} \frac{d\omega}{2\pi} e^{-i(\omega+m\Omega)t+i(\omega+n\Omega)t'} \left[ \overline{G^R(\omega)} \right]_{mn}. \quad (19)$$

Using  $\left[ \overline{G^R(\omega)} \right]_{(m+s)(n+s)} = \left[ \overline{G^R(\omega + s\Omega)} \right]_{mn}$ , one can obtain the propagator starting from  $t_0 = 0$

$$G^R(t, 0) = \sum_{n=-\infty}^{\infty} \int_{-\infty}^{\infty} \frac{d\omega}{2\pi} e^{-i\omega t} \left[ \overline{G^R(\omega)} \right]_{n0}. \quad (20)$$

Eq. 17, 18 and 20 are the main results of this section. In the following contents, we will analysis their behaviors.

### A. The definition of lifetime

#### 1. Review the definition of lifetime based on the Green's function

We first review the definition of lifetime based on the Green's function method. Consider a free electron with energy dispersion  $E(k)$ , the corresponding retarded Green's function can be defined as

$$G_0^R(k, \omega) = \frac{1}{\omega - E(k) + i\eta^+}, \quad (21)$$

where  $\eta^+ = 0^+$ . Therefore, the corresponding propagator becomes

$$G_0(t) = \sum_k \int_{-\infty}^{\infty} \frac{\omega}{2\pi} e^{-i\omega t} G_0^R(k, \omega) \propto \sum_k e^{iE(k)t - \eta^+ t}. \quad (22)$$

Here each  $k$  corresponds to a quasiparticle mode. When  $\eta^+ > 0$ , the propagator will decay with time, and defines a corresponding lifetime. We note that in the non-interacting isolated systems,  $\eta = 0^+$ , which means the quasiparticle lifetime is infinity.

Generalizing the above argument to the interacting or open quantum systems, the retarded Green's becomes

$$G^R(k, \omega) = \frac{1}{\omega - E(k) - \Sigma(\omega)}. \quad (23)$$

A standard statement of the lifetime is that the imaginary part of the pole corresponds to the lifetime. Namely, consider

$$\omega - E(k) - \Sigma(\omega) = \frac{\prod_{n=1}^m [\omega - \varepsilon_n(k) + i\Gamma_n(k)]}{D(\omega)}, \quad (24)$$

the propagator becomes

$$G(t) = \sum_k \int_{-\infty}^{\infty} \frac{\omega}{2\pi} e^{-i\omega t} G^R(k, \omega) \propto \sum_n \sum_k D[\varepsilon_n(k) - i\Gamma_n(k)] e^{i\varepsilon_n(k)t - \Gamma_n(k)t}. \quad (25)$$

Here  $D[\varepsilon_n(k) - i\Gamma_n(k)]$  describes the quasiparticle weight, and the quasiparticle lifetime is modified by the self-energy induced by interacting or external environment, and the additional degrees  $n$  correspond to the additional quasiparticles provided by the external environment.

We note that the above argument implies  $\omega - E(k) - \Sigma(\omega)$  is proportional to an algebraic equation. However, in general, the external environment degrees are infinity, which renders that the self-energy is not an algebraic polynomial (just like our Majorana poisoning model). In this case, can we generalize the above method directly?

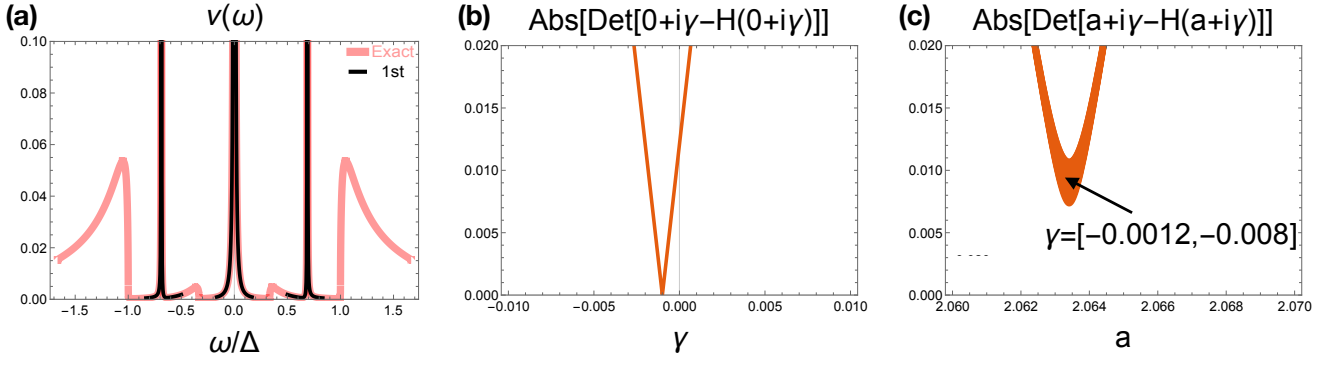

FIG. 2. The peaks and poles in the Floquet Majorana poisoning model. (a) shows the numerical calculation of  $\nu(\omega)$  in Eq. 26 with  $\Omega = 2$ ,  $\Delta = 3$ ,  $A = 1/2$ ,  $\eta = 1/1000$  and  $V = 1$ . (b) and (c) shows the function  $\text{Abs}[\det[\omega - H(\omega)]]$  around the peaks at  $\omega = 0$  and  $\omega \simeq 2.064$ .

## 2. Some insights of the Majorana poisoning model

We first apply the above method to the Majorana poisoning model directly, and see what happens. In order to simplify the discussion, we assume  $N_F = 1$ . In this case,

$$\underline{\omega} - \underline{H}(\omega) = \begin{pmatrix} (\omega + \Omega) - \Sigma(\omega + \Omega) & -A & 0 \\ -A & \omega - \Sigma(\omega) & -A \\ 0 & -A & (\omega - \Omega) - \Sigma(\omega - \Omega) \end{pmatrix}. \quad (26)$$

$\nu(\omega)$  is plotted in Fig. 2 (a) with the following parameters  $\Omega = 2$ ,  $\Delta = 3$ ,  $A = 1/2$ ,  $\eta = 1/1000$ , where there only exist three in-gap peaks.

Importantly, we numerical solve the following equation

$$\det[\underline{\omega} - \underline{H}(\omega)] = 0 \quad (27)$$

and find that there only exist one solution,  $\omega = 0 + i\eta$ . Another way to verify this is to plot the function  $\text{Abs}[\det[\underline{\omega} - \underline{H}(\omega)]]$ . Since there exist a peak around  $\omega = 0, \pm 2$ , we plot the function  $\text{Abs}[\det[\underline{\omega} - \underline{H}(\omega)]]$  around them. As shown in Fig. 2 (b), we plot  $\text{Abs}[\det[\underline{\omega} - \underline{H}(\omega)]]$  with  $\omega = 0 + i\gamma$ . One can find it becomes zero at  $\gamma = -\eta$ . However, when we plot the function  $\text{Abs}[\det[\underline{\omega} - \underline{H}(\omega)]]$  around  $\omega = 2$  in the complex  $\omega$  plane, namely,  $\Re[\omega] \in [2.06, 2.07]$  and  $\Im[\omega] \in [-0.0012, -0.008]$ , the function  $\text{Abs}[\det[\underline{\omega} - \underline{H}(\omega)]]$  does not become zero. We note that due to finite  $N_F$  namely,  $N_F = 1$ , the peaks in the second Floquet BZ does not at  $\omega = \pm 2$  exactly, but around  $\omega = 2.064$ . That's the reason why we chose the plot region in (c).

Although  $\det[\underline{\omega} - \underline{H}(\omega)] = 0$  does not have poles around  $\omega = \pm 2$  in the complex  $\omega$  plane, these peaks can be well fitted by the following method.

1. Expand the Hamiltonian 26 around  $\omega = 0, \pm\Omega$  up to linear order. For example,

$$\begin{aligned} \underline{\omega} - \underline{H}(\omega) &\simeq -\underline{H}(0) + [\delta\omega - \underline{H}^{(1)}(0, \delta\omega)] \\ &= -\underline{H}(0) + \left[ \delta\omega - \begin{pmatrix} -\Sigma^{(1)}(\Omega)\delta\omega & 0 & 0 \\ 0 & -\Sigma^{(1)}(0)\delta\omega & 0 \\ 0 & 0 & -\Sigma^{(1)}(-\Omega)\delta\omega \end{pmatrix} \right], \end{aligned} \quad (28)$$

where

$$\Sigma^{(1)}(m\Omega) = \frac{d}{d\omega} \Sigma^{(1)}(\omega)|_{\omega=m\Omega}. \quad (29)$$

Notice that the linear term of  $\delta\omega$  in the above matrix are not proportional to the identity matrix due to the fact that  $\Sigma^{(1)}(\pm\Omega) \neq \Sigma^{(1)}(0)$ .

2. Using the expansion Hamiltonian to express the Green's function, for example,

$$\underline{G}^R(\omega) = \frac{1}{\underline{\omega} - \underline{H}(\omega)} \simeq \frac{1}{-\underline{H}(0) + [\delta\omega - \underline{H}^{(1)}(0, \delta\omega)]}. \quad (30)$$

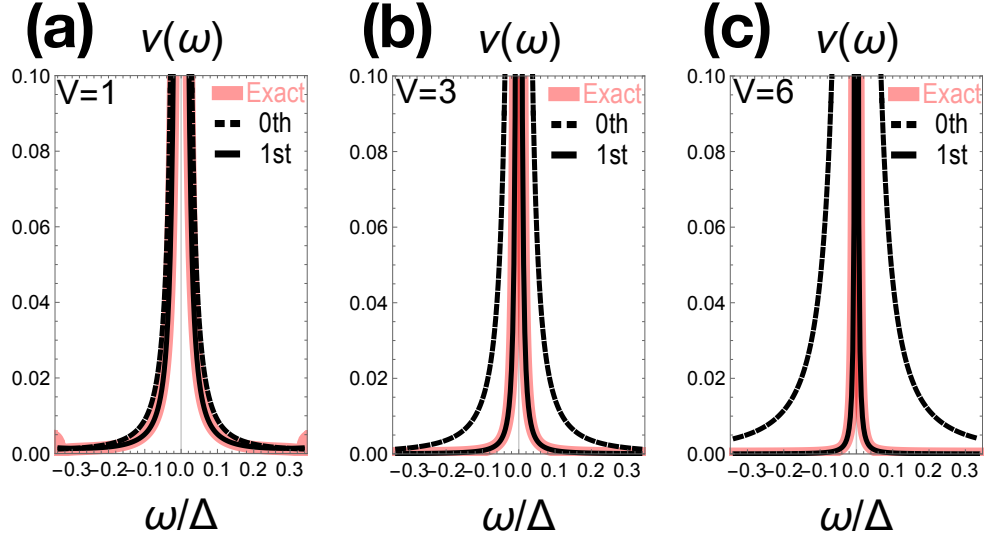

FIG. 3. Floquet Majorana poisoning model. (a)-(c) show the exact, zeroth and first order numerical calculation of  $\nu(\omega)$  in Eq. 18 with  $\Omega = 2$ ,  $\Delta = 3$ ,  $A = 1/2$ ,  $\eta = 1/1000$ ,  $N_F = 10$ , and different values of  $V$ .

3. Using the approximated Green's function to calculate the DoS. For example,

$$\nu(\omega) = -\frac{1}{\pi} \text{Im} \left[ \overline{G^R(\omega)} \right]_{00} \simeq -\frac{1}{\pi} \text{Im} \left[ \frac{1}{-\underline{H}(0) + \left( \underline{\delta\omega} - \underline{H^{(1)}(0, \delta\omega)} \right)} \right]_{00}. \quad (31)$$

As shown in Fig. 2, the first order approximation are plotted with black lines. One can find that they match the exact solutions very well.

We also note that in some discussion, the expansion around  $\omega = 0$  is applied up to the zeroth order, and obtain an effective Hermitian or non-Hermitian Hamiltonian, namely,

$$H_{eff}(k) \simeq H_0(k) + \Sigma^{(0)}(k, \omega = 0). \quad (32)$$

The corresponding real and imaginary parts of the complex eigenvalues of  $H_{eff}$  represent the renormalized band dispersion and quasiparticle lifetime. However, this approach also fails in our model. As shown in Fig. 3 (a)-(c), the exact/first order/second order results of the time-averaged DoS are plotted around  $\omega = 0$  with the red/dashed black/solid black lines, respectively. One can notice from Fig. 3 (a)-(c) that with the increasing of  $V$ , the zeroth order breaks down, while the first order approximation works well. When the expansion is applied around  $\omega_0 = m\Omega$  up to linear order, one can use the same method to fix the order peaks as shown in Fig. 3 (c) the main text.

Based on the above analysis, although we find that the traditional method does not work here due to the absence of poles around  $\omega = \pm\Omega$ , the peaks around them can be approximated by the first order expansion.

### 3. Definition of lifetime

The triumph of the first order approximation is related to the definition of lifetime. As mentioned above,  $\det[\omega - H(\omega)]$  can not be expressed as a finite set of product of  $\omega - E_n$  without any approximation. However, when we expand the Hamiltonian around  $\omega_0$ , the determinant of inverse of the Green's function becomes an algebraic polynomial. As a result, one can find the corresponding poles around  $\omega_0$ . Based on this spirit, the corresponding lifetime is defined as the imaginary part of the poles around  $\omega_0$ . Now we summarize the procedure to calculate the lifetime.

1. Expand  $\underline{\omega} - \underline{H}(\omega)$  around  $\omega = m\Omega$ ,

$$\underline{\omega} - \underline{H}(\omega) \simeq \underline{\omega}_0 - \underline{H}^{(0)}(\omega_0) + \underline{\delta\omega} - \underline{H}^{(1)}(\omega_0, \delta\omega) - o(\delta\omega^2), \quad (33)$$

where  $\delta\omega = \omega - \omega_0$ , and  $\underline{H}^{(i)}(\omega_0, \delta\omega^i)$  is a matrix only containing  $\delta\omega^i$  term.

2. Calculate the following equation

$$\det \left[ \underline{\omega}_0 - \underline{H}^{(0)}(\omega_0) + \underline{\delta\omega} - \underline{H}^{(1)}(\omega_0, \delta\omega) \right] \simeq f_0 + f_1 \delta\omega + o(\delta\omega^2). \quad (34)$$

3. Then the lifetime of the quasiparticle around  $\omega = \omega_0$  is

$$\Gamma_{\omega_0} = -\frac{1}{\Im[f_0/f_1]}. \quad (35)$$

Notice that the above procedure is equivalent to

$$\det \left[ \underline{\omega} - \underline{H}(\omega) \right] \simeq f_0(\omega_0) + f_1(\omega_0) \delta\omega + o(\delta\omega^2). \quad (36)$$

However, the direct calculation of  $\det[\underline{\omega} - \underline{H}(\omega)]$  is not easy in numerics.

### B. The lifetime of the Floquet Majoranas in different Floquet BZs

Now we show that all the quasiparticles in different Floquet BZs have the same lifetime. We notice that due to the discrete time translational symmetry, we have

$$\det \left[ \underline{\omega} - \underline{H}(\omega) \right] = \det \left[ (\omega + m\Omega) - \underline{H}(\omega + m\Omega) \right]. \quad (37)$$

Therefore, the expansion of  $\det[\underline{\omega} - \underline{H}(\omega)]$  around  $\omega = m\Omega$  must share the same expression. Therefore, their lifetimes are the same. This is consistent with the intuition, since the total Hamiltonian does not break the discrete time translational symmetry.

### C. The differences between the peaks in different Floquet BZs

This section explains the differences between the FMZMs in different Floquet bands. We start from the  $mn$ -entry of the retarded Green's function

$$\left[ \underline{G}^R(\omega) \right]_{mn} = \langle m | \frac{1}{\underline{\omega} - \underline{H}(\omega)} | n \rangle = \sum_s \frac{\langle m | u_s^R(\omega) \rangle \langle u_s^L(\omega) | n \rangle}{\omega - E_s(\omega)}. \quad (38)$$

Here  $\underline{H}(\omega) | u_s^R(\omega) \rangle = E_s(\omega) | u_s^R(\omega) \rangle$ ,  $\langle u_s^L(\omega) | \underline{H}^\dagger(\omega) = E_s(\omega) \langle u_s^L(\omega) |$ , and  $\langle u_n^L(\omega) | u_m^R(\omega) \rangle = \delta_{nm}$  is the biorthogonal basis. The time-averaged DoS is defined by

$$\nu(\omega) = -\frac{1}{\pi} \text{Im} \left[ \underline{G}^R(\omega) \right]_{00} = -\frac{1}{\pi} \text{Im} \left[ \sum_s \frac{\langle 0 | u_s^R(\omega) \rangle \langle u_s^L(\omega) | 0 \rangle}{\omega - E_s(\omega)} \right]. \quad (39)$$

As discussed in the main text, the wavefunctions  $\langle 0 | u_s^R(\omega) \rangle$  are localized in the central part of the Floquet base. Therefore, the DoS will decay in the higher Floquet BZs.

- 
- [1] H. Aoki, N. Tsuji, M. Eckstein, M. Kollar, T. Oka, and P. Werner, *Rev. Mod. Phys.* **86**, 779 (2014).
  - [2] J. Rammer and H. Smith, *Rev. Mod. Phys.* **58**, 323 (1986).
  - [3] V. Chandrasekhar, “An introduction to the quasiclassical theory of superconductivity for diffusive proximity-coupled systems,” (2003), [arXiv:cond-mat/0312507 \[cond-mat.mes-hall\]](#).
  - [4] D. J. Thouless and S. Kirkpatrick, *Journal of Physics C: Solid State Physics* **14**, 235 (1981).
  - [5] P. A. Lee and D. S. Fisher, *Phys. Rev. Lett.* **47**, 882 (1981).
  - [6] P. S. Drouvelis, P. Schmelcher, and P. Bastian, *Journal of Computational Physics* **215**, 741 (2006).
